# Supplementary material for: Recursive Compressed Sensing
Source: arXiv:1312.4895 source file (2013-12-17)
Supplement: Supplementary file 1 [file appendix.tex]

\section{Appendix}
\label{sec:appendix}

\subsection{Deviation from Expected Signal Sparsity}

In this section we study $\E\left[\Vert \X-\X_\kappa \Vert_1\right]$ where the elements of random vector $\X \in \R^n$ are chosen i.i.d. having probability density 
\begin{align}
f_{X_i}(x) =
\begin{cases}
(1-p)\delta(x) + \frac{1}{2p} &\mbox{if } x \in [-1,1] \\
0 & \mbox{o.w. }
\end{cases}
\label{eq:signal_model}
\end{align}
where $p \in \left[0,1\right]$. This is the density function of a random variable that is $0$ with probability $1-p$ and sampled uniformly over the interval $[-1,1]$ otherwise.

Based on this the probability of $\X$ having exactly $k$ nonzero values is
\begin{align*}
P\left( \Vert \X \Vert_0 = k \right) = {n \choose k} p^k (1-p)^{n-k}.
\end{align*}

Let $\Zv$ be the random vector obtained by ordering the nonzero elements of $\X$ in descending order with respect to the magnitude, i.e., $Z_i$ is equal to the $i^{th}$ greatest element of $\vert \X \vert$. With this definition we have $\Zv \in \R^{\Vert X \Vert_0}$ and probability that $Z_i$ is less than $T$ equals to
\begin{align}
P({Z_i < T \mid \Vert \X \Vert_0=k}) = \sum_{m = 0}^{i-1} {k \choose m} P(X_1 \geq T)^m P(X_1 <T)^{k-m}.
\label{eq:pdfzt}
\end{align}
This value is also equivalent to the probability of having at most $i-1$ elements of $\Zv$ being greater than or equal to $T$. From this we find
\begin{align}
f_{{Z_i \mid k}}(T) = \frac{d}{dT} P({Z_i < T \mid \Vert \X \Vert_0=k}).
\label{eq:pdf_}
\end{align}

We then note that
\begin{align*}
\E\left[\Vert \X-\X_\kappa \Vert_1\right] &= \E\left[ \vert Z_{\kappa+1} \vert+ \vert Z_{\kappa+2}\vert + \cdots + \vert Z_{n} \vert \right] \\
 &= P\left(\Vert \X \Vert_0 = \kappa+1\right) \E\left[ Z_{\kappa+1} | \Vert X \Vert_0 = \kappa+1 \right] \\
 & + P\left(\Vert \X \Vert_0 = \kappa+2\right) \E\left[ Z_{\kappa+1} + Z_{\kappa+2} | \Vert \X \Vert_0 = \kappa+2 \right] \\
 & + \dots \\
 & + P\left(\Vert \X \Vert_0 = n\right) \E\left[ \sum_{i=\kappa+1}^{n} Z_{i} | \Vert \X \Vert_0 = n \right] \\
 &= \sum_{j = \kappa+1}^{n} P\left(\Vert \X \Vert_0 = j\right) \E\left[ \sum_{i=\kappa+1}^{j} Z_{i} | \Vert \X \Vert_0 = j \right]
\end{align*}.

In our case, since the nonzero elements of $\X$ is $X_i \sim \mathcal{U}\left( \left[ -1, 1 \right] \right)$ we have $P(X_1 < T) = T$, substituting this into \eqref{eq:pdfzt} yields
\begin{align*}
P({Z_i < T \mid \Vert \X \Vert_0=k}) = \sum_{m = 0}^{i-1} {k \choose m} (1-T)^m (T)^{k-m}
\end{align*}
using this in \eqref{eq:pdf_} and simplifying the terms we have
\begin{align*}
f_{{Z_i \mid k}}(T) = \sum_{m=0}^{i-1} {k \choose m} (1-T)^{m-1} T^{k-m-1} \left(  k - m -kT \right).
\end{align*}.

We find the expected value of $Z_i$ as
\begin{align*}
\E\left[{\vert Z_i \vert \mid \Vert X \Vert_0=k}\right] &= \int_0^1 Tf_{Z_i\vert k}(T) \,dT \\
&= \int_0^1 \sum_{m=0}^{i-1} {k \choose m} (1-T)^{m-1} T^{k-m} \left(  k - m -kT \right) \,dT \\
&= 1 - \sum_{m=0}^{i-1} \frac{1}{k+1} \\
&= 1 - \frac{i}{k+1} 
\end{align*}

Denoting the signal obtained by taking elements of $\Zv$ having indices more than $\kappa$, $\Zv_{i>\kappa} := \begin{bmatrix}Z_{\kappa+1} & Z_{\kappa+2} & \dots & Z_{k}\end{bmatrix}$ we have:

\begin{align*}
 \E\left[{\Vert \Zv_{i>\kappa} \Vert_1 \mid \Vert X \Vert_0 = k}\right]&= \sum_{i = \kappa+1}^{k} \E\left[{\vert Z_i \vert \mid \Vert \X \Vert_0=k}\right]\\ 
&= \sum_{i=\kappa+1}^{k} \left( 1 - \frac{i}{k+1} \right)
\end{align*}

Then we use the towering property of conditional expectation 
\begin{align*}
\ev{\Vert \X-\X_\kappa \Vert_1} &= \E \left[ \Vert \Zv_{i>\kappa} \Vert_1 \right] \nonumber \\
&= \E \left[   \E\left[{\Vert \Zv_{i>\kappa} \Vert_1 \mid \Vert \X \Vert_0}\right] \right] \nonumber \\
&= \sum_{k=\kappa+1}^{n} P(\Vert \X \Vert_0 =k)   \ev{\Vert \Zv_{i>\kappa} \Vert_1 \mid \Vert \X \Vert_0 = k}  \nonumber \\
&=  \sum_{k=\kappa+1}^{n} {n \choose k} p^k (1-p)^{n-k} \sum_{i=\kappa+1}^{k} \left( 1 - \frac{i}{k+1} \right)
\end{align*}

The result is a function of the signal length, $n$, the number of elements we look at, $\kappa$, and the probability of getting a nonzero element, $p$.

Two plots showing the deviation from expected signal sparsity are depicted in Figure \ref{fig:expected_norm_plots}. For small probabilities, the norm of $\ev{\Vert \X-\X_\kappa \Vert_1}$ starts out low, but as the window length increase $\ev{\Vert \X-\X_\kappa \Vert_1}$ becomes higher for small values of $p$.

\begin{figure*}[!t]
        \centering
        \begin{subfigure}[h]{0.48\linewidth}
                \centering
                \includegraphics[width = \linewidth]{images/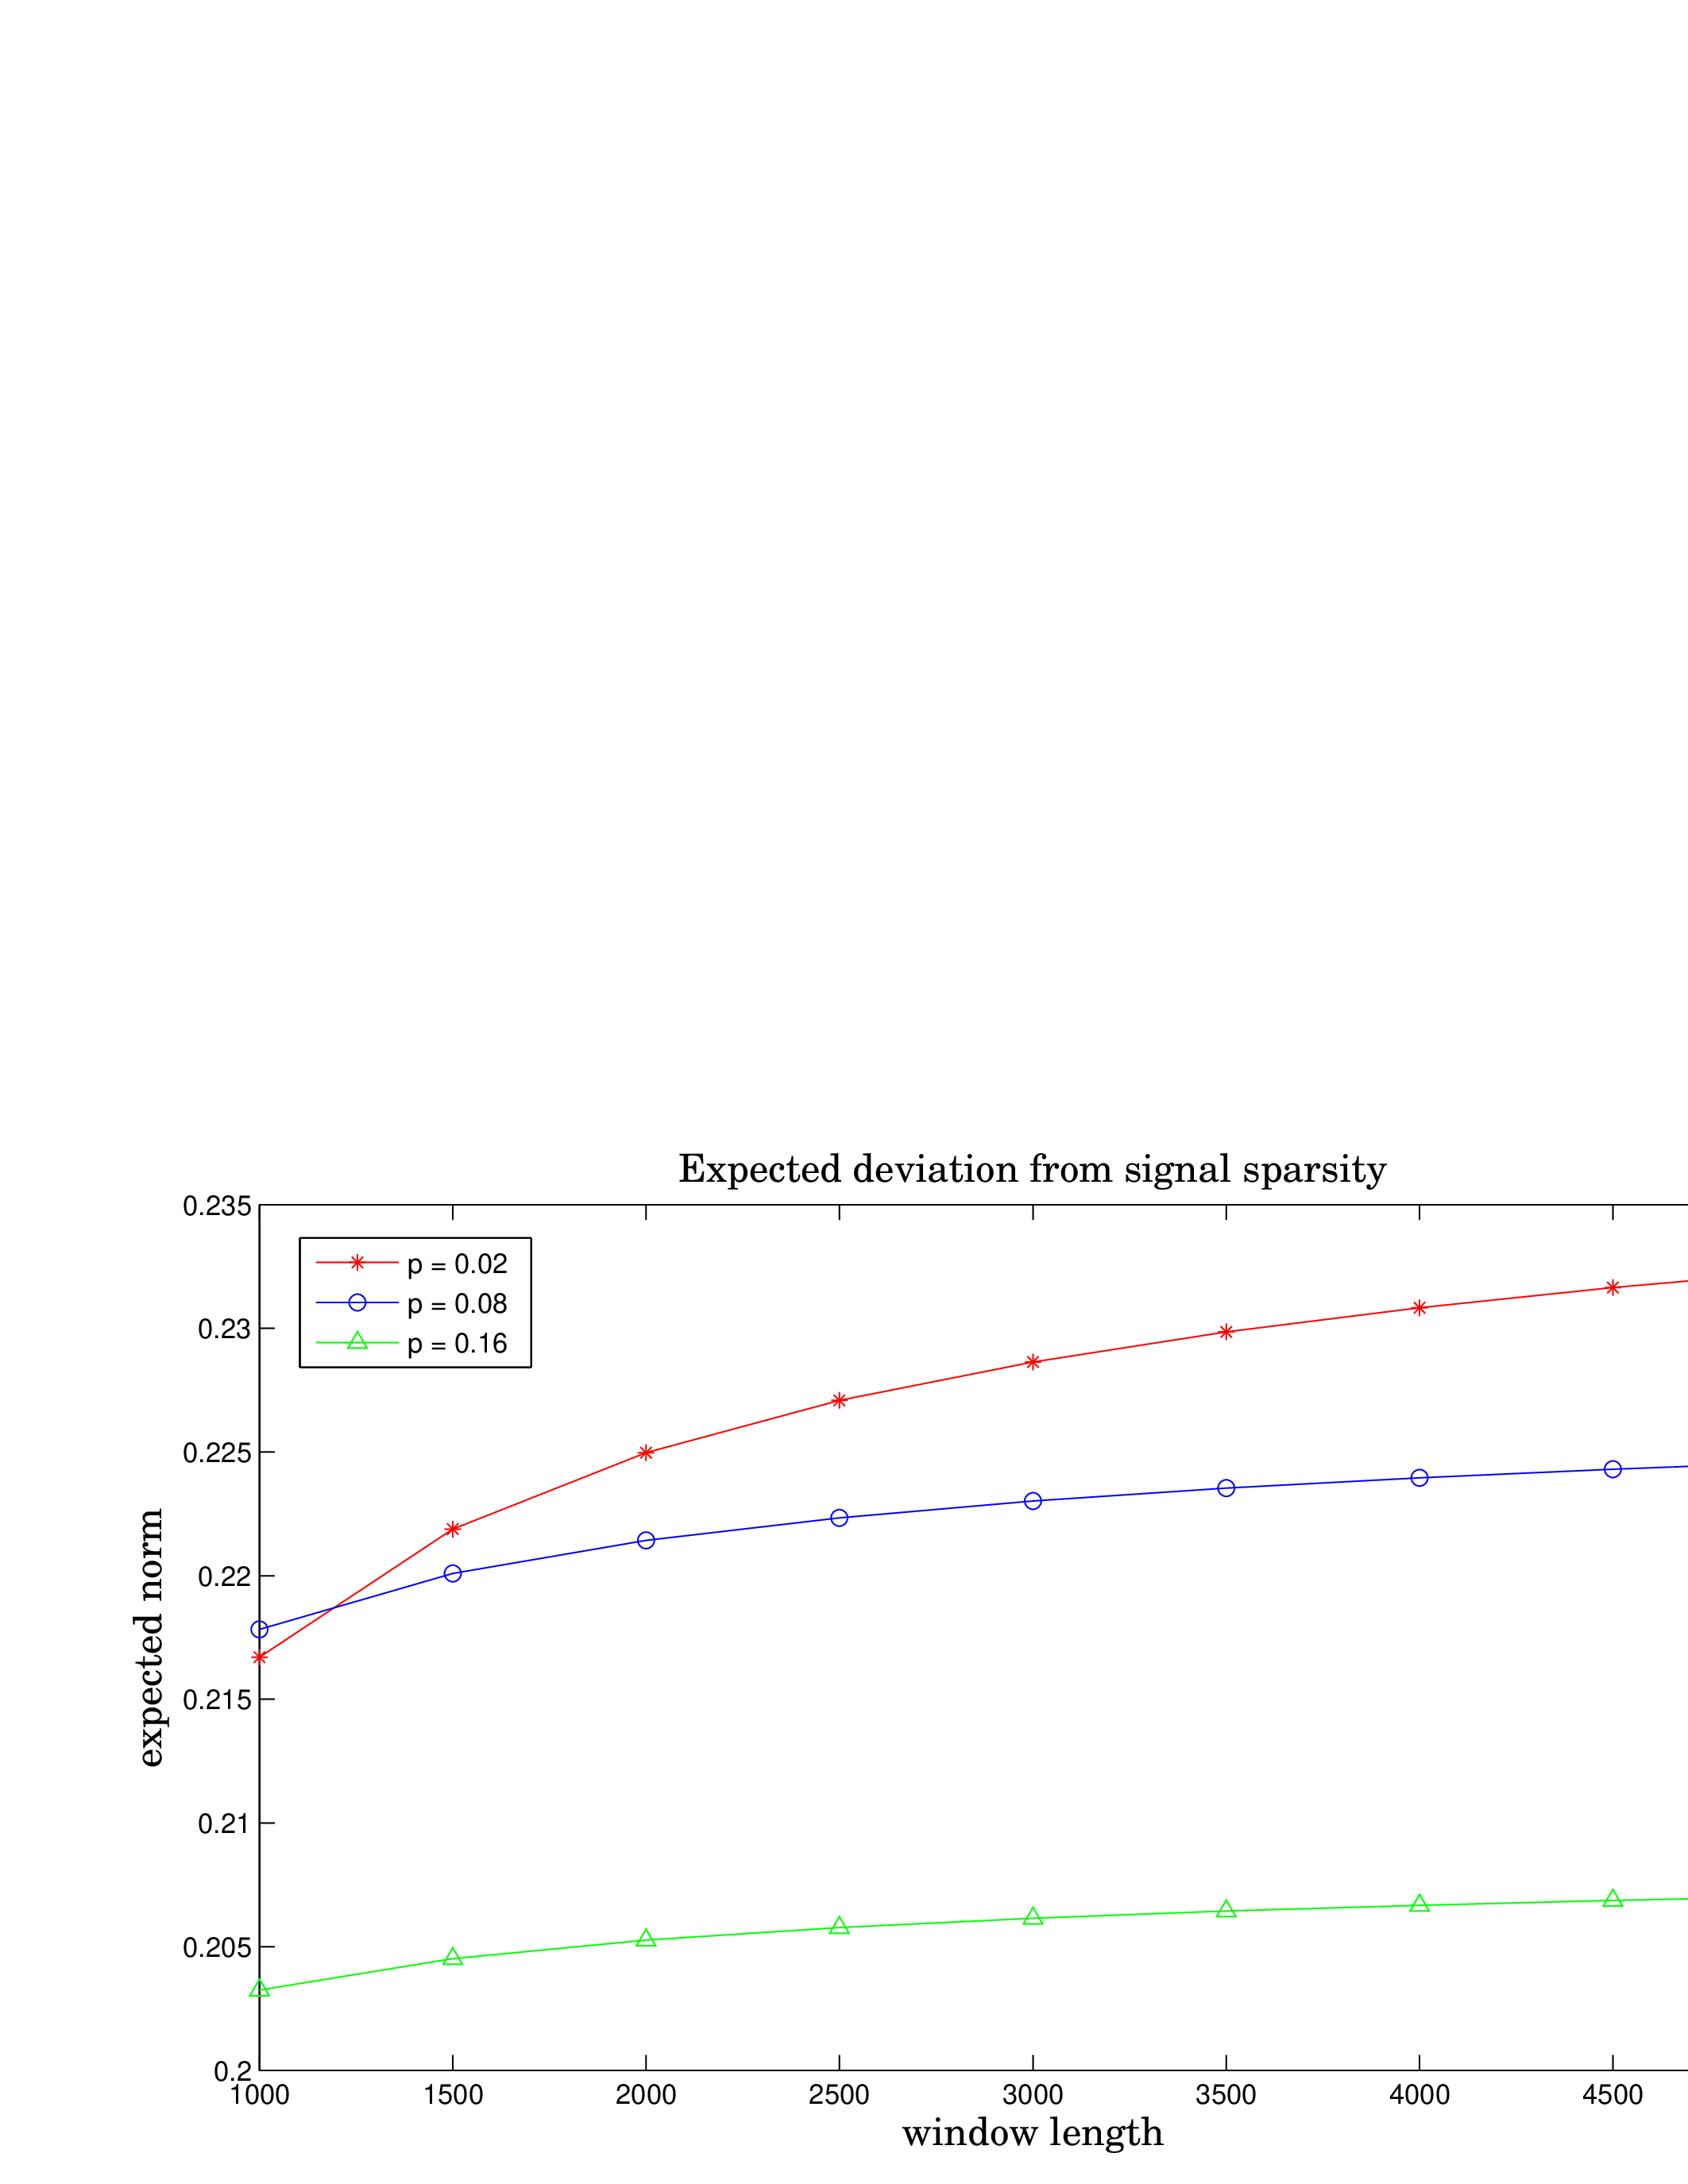}
                \caption{Expected deviation from signal sparsity, $\ev{\Vert \X-\X_\kappa \Vert_1}$, for $\kappa = np$ vs. the window length.}
                \label{fig:norm_expected1}
        \end{subfigure}
        \quad
        \begin{subfigure}[h]{0.48\linewidth}
                \centering
                \includegraphics[width = \linewidth]{images/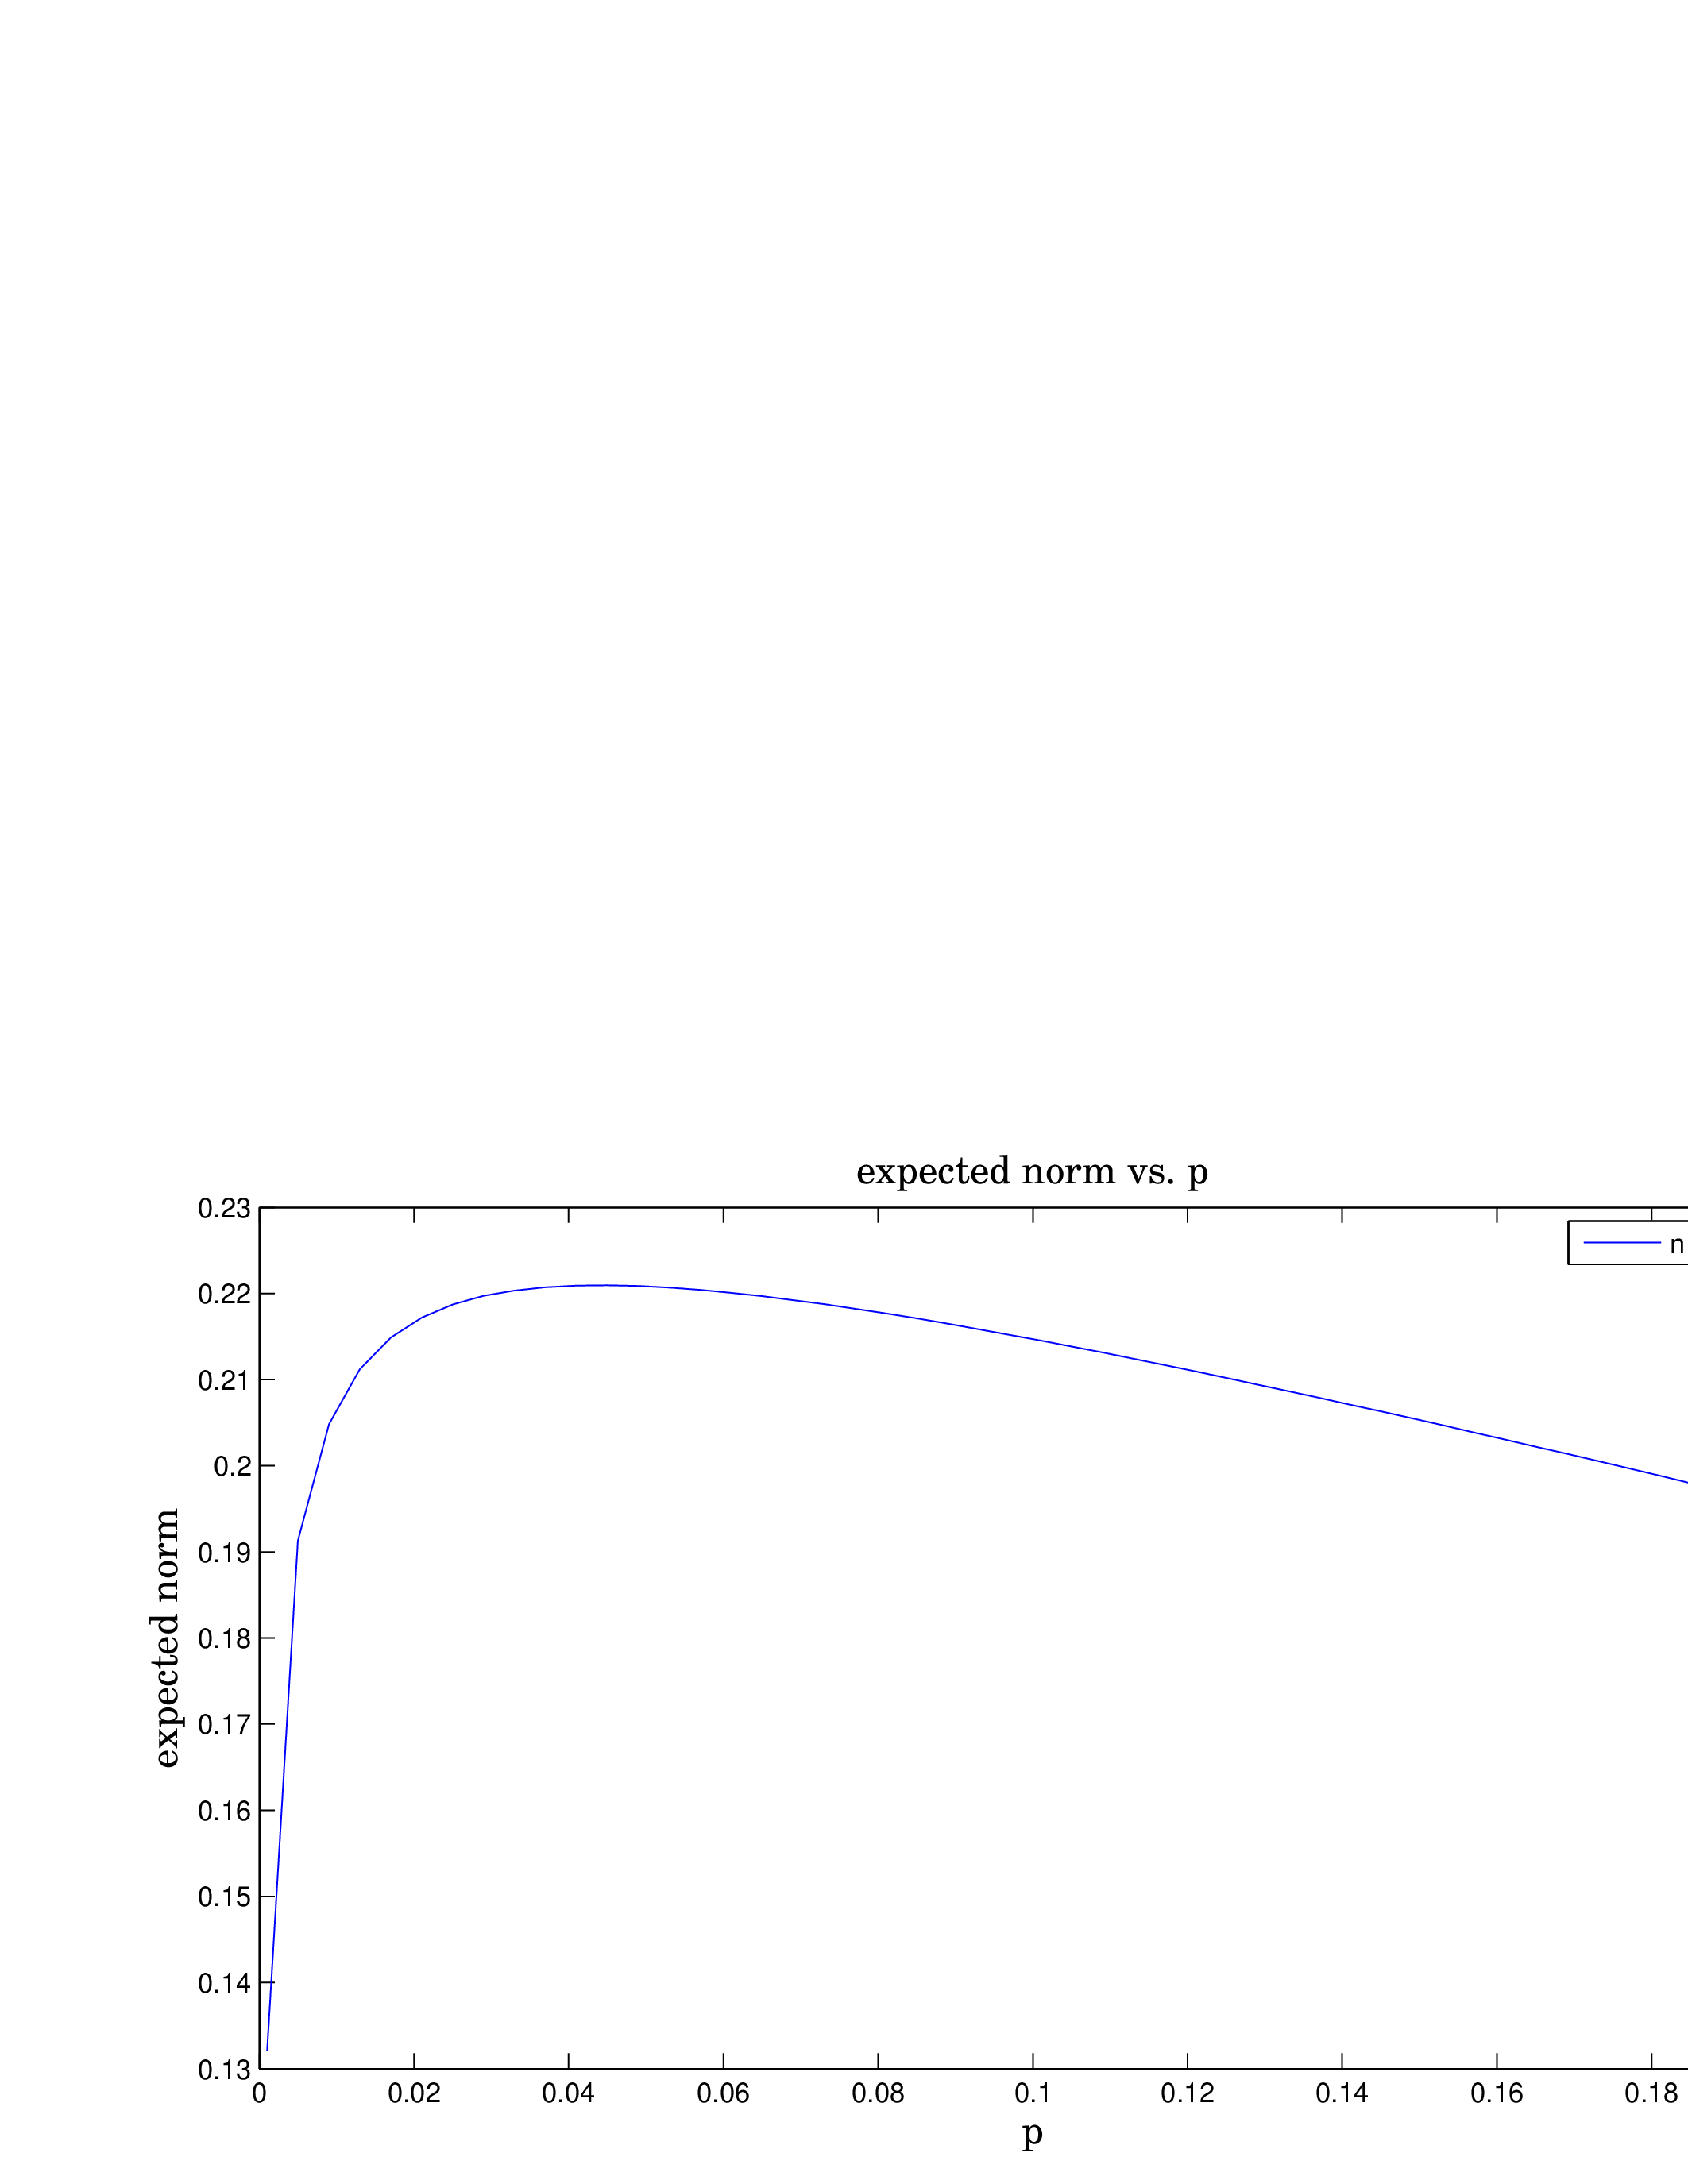}
                \caption{Expected deviation from signal sparsity, $\ev{\Vert \X-\X_\kappa \Vert_1}$, for $\kappa = np$, $n = 1000$ vs. $p$.}
                \label{fig:norm_expected2}
        \end{subfigure}
        \caption{Figures for deviation from expected signal sparsity, $\ev{\Vert \X-\X_\kappa \Vert_1}$, given the signal model in \eqref{eq:signal_model}.}
        \label{fig:expected_norm_plots}
\end{figure*}
